# Supplementary material for: The Illusion of Randomness: An Empirical Analysis of Address Space Layout Randomization Implementations
Source: arXiv:2408.15107 source file (2024-08-29)
Supplement: Supplementary file 1 [file linux.tex]

\section{Linux Results}
\begin{figure*}[tbh]
    \begin{adjustwidth}{-1.6cm}{-1.6cm}
    \centering
    \begin{subfigure}[t]{0.57\textwidth}
        \centering
        \includegraphics[width=\textwidth]{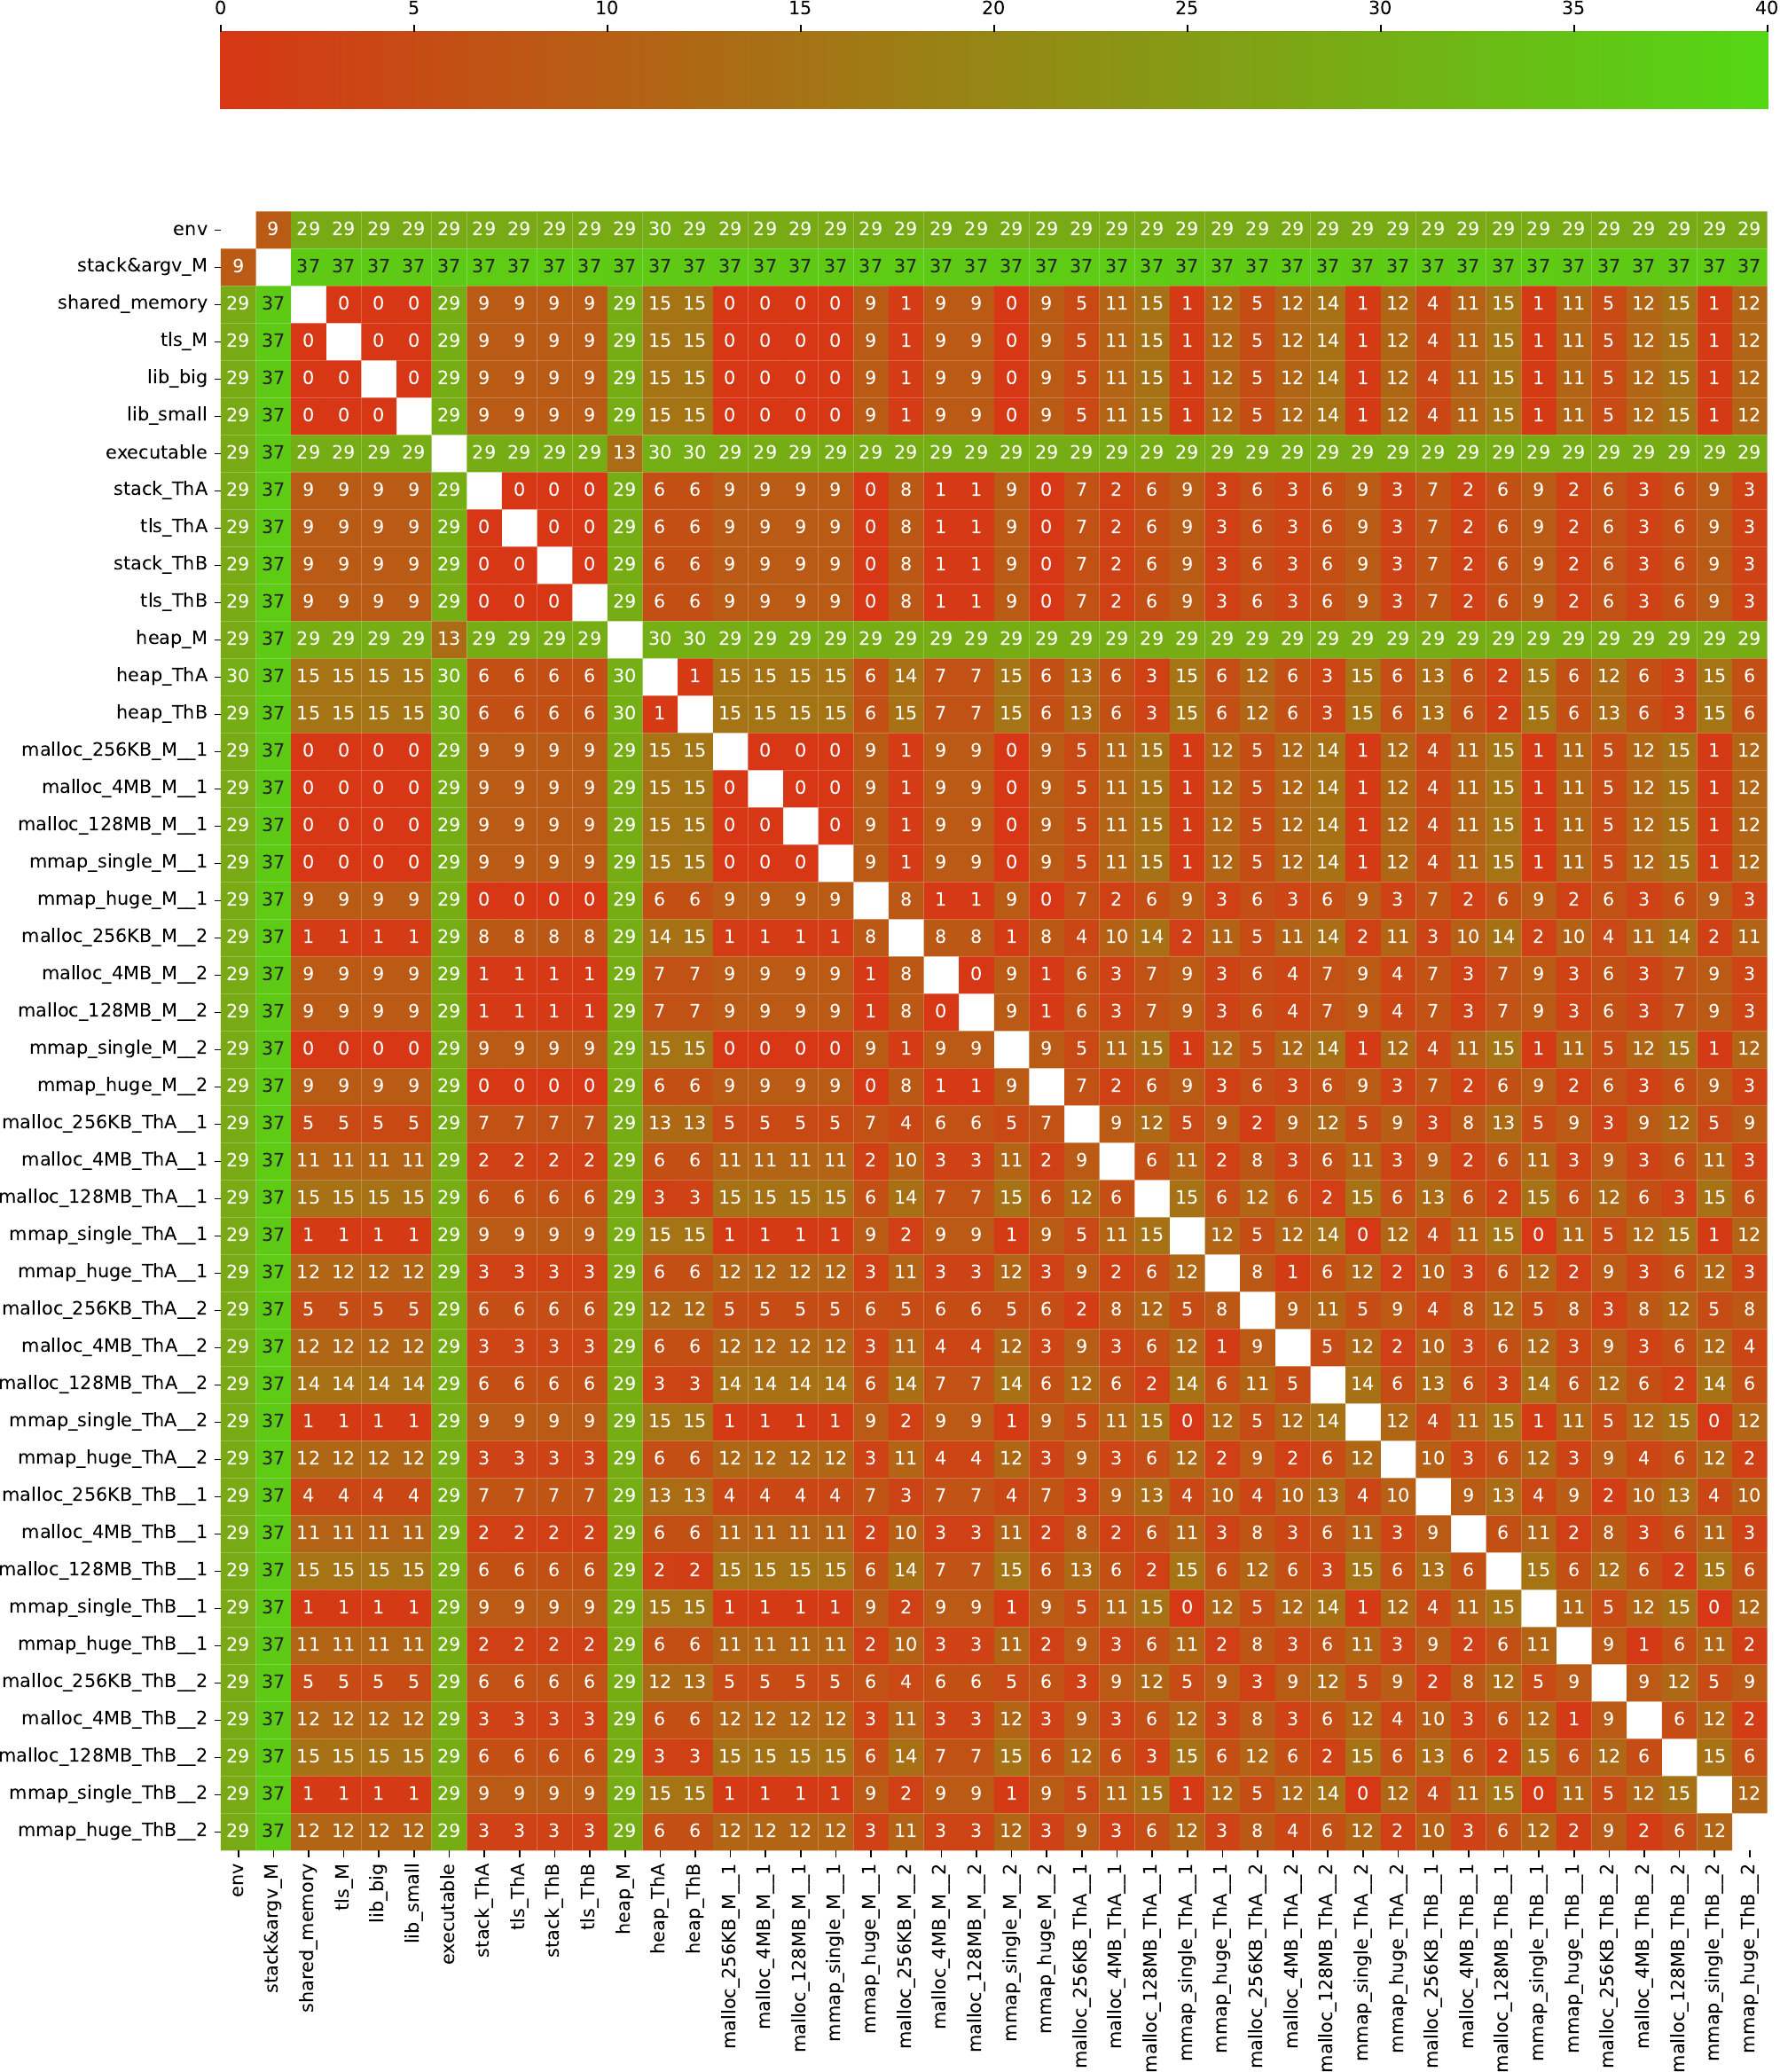}
        \caption{Correlation Entropy Linux 5.17.19}
        \label{fig:corr_lin517}
    \end{subfigure}%
    \hfill % Ensures that there is no additional space between the figures
    \begin{subfigure}[t]{0.57\textwidth}
        \centering
        \includegraphics[width=\textwidth]{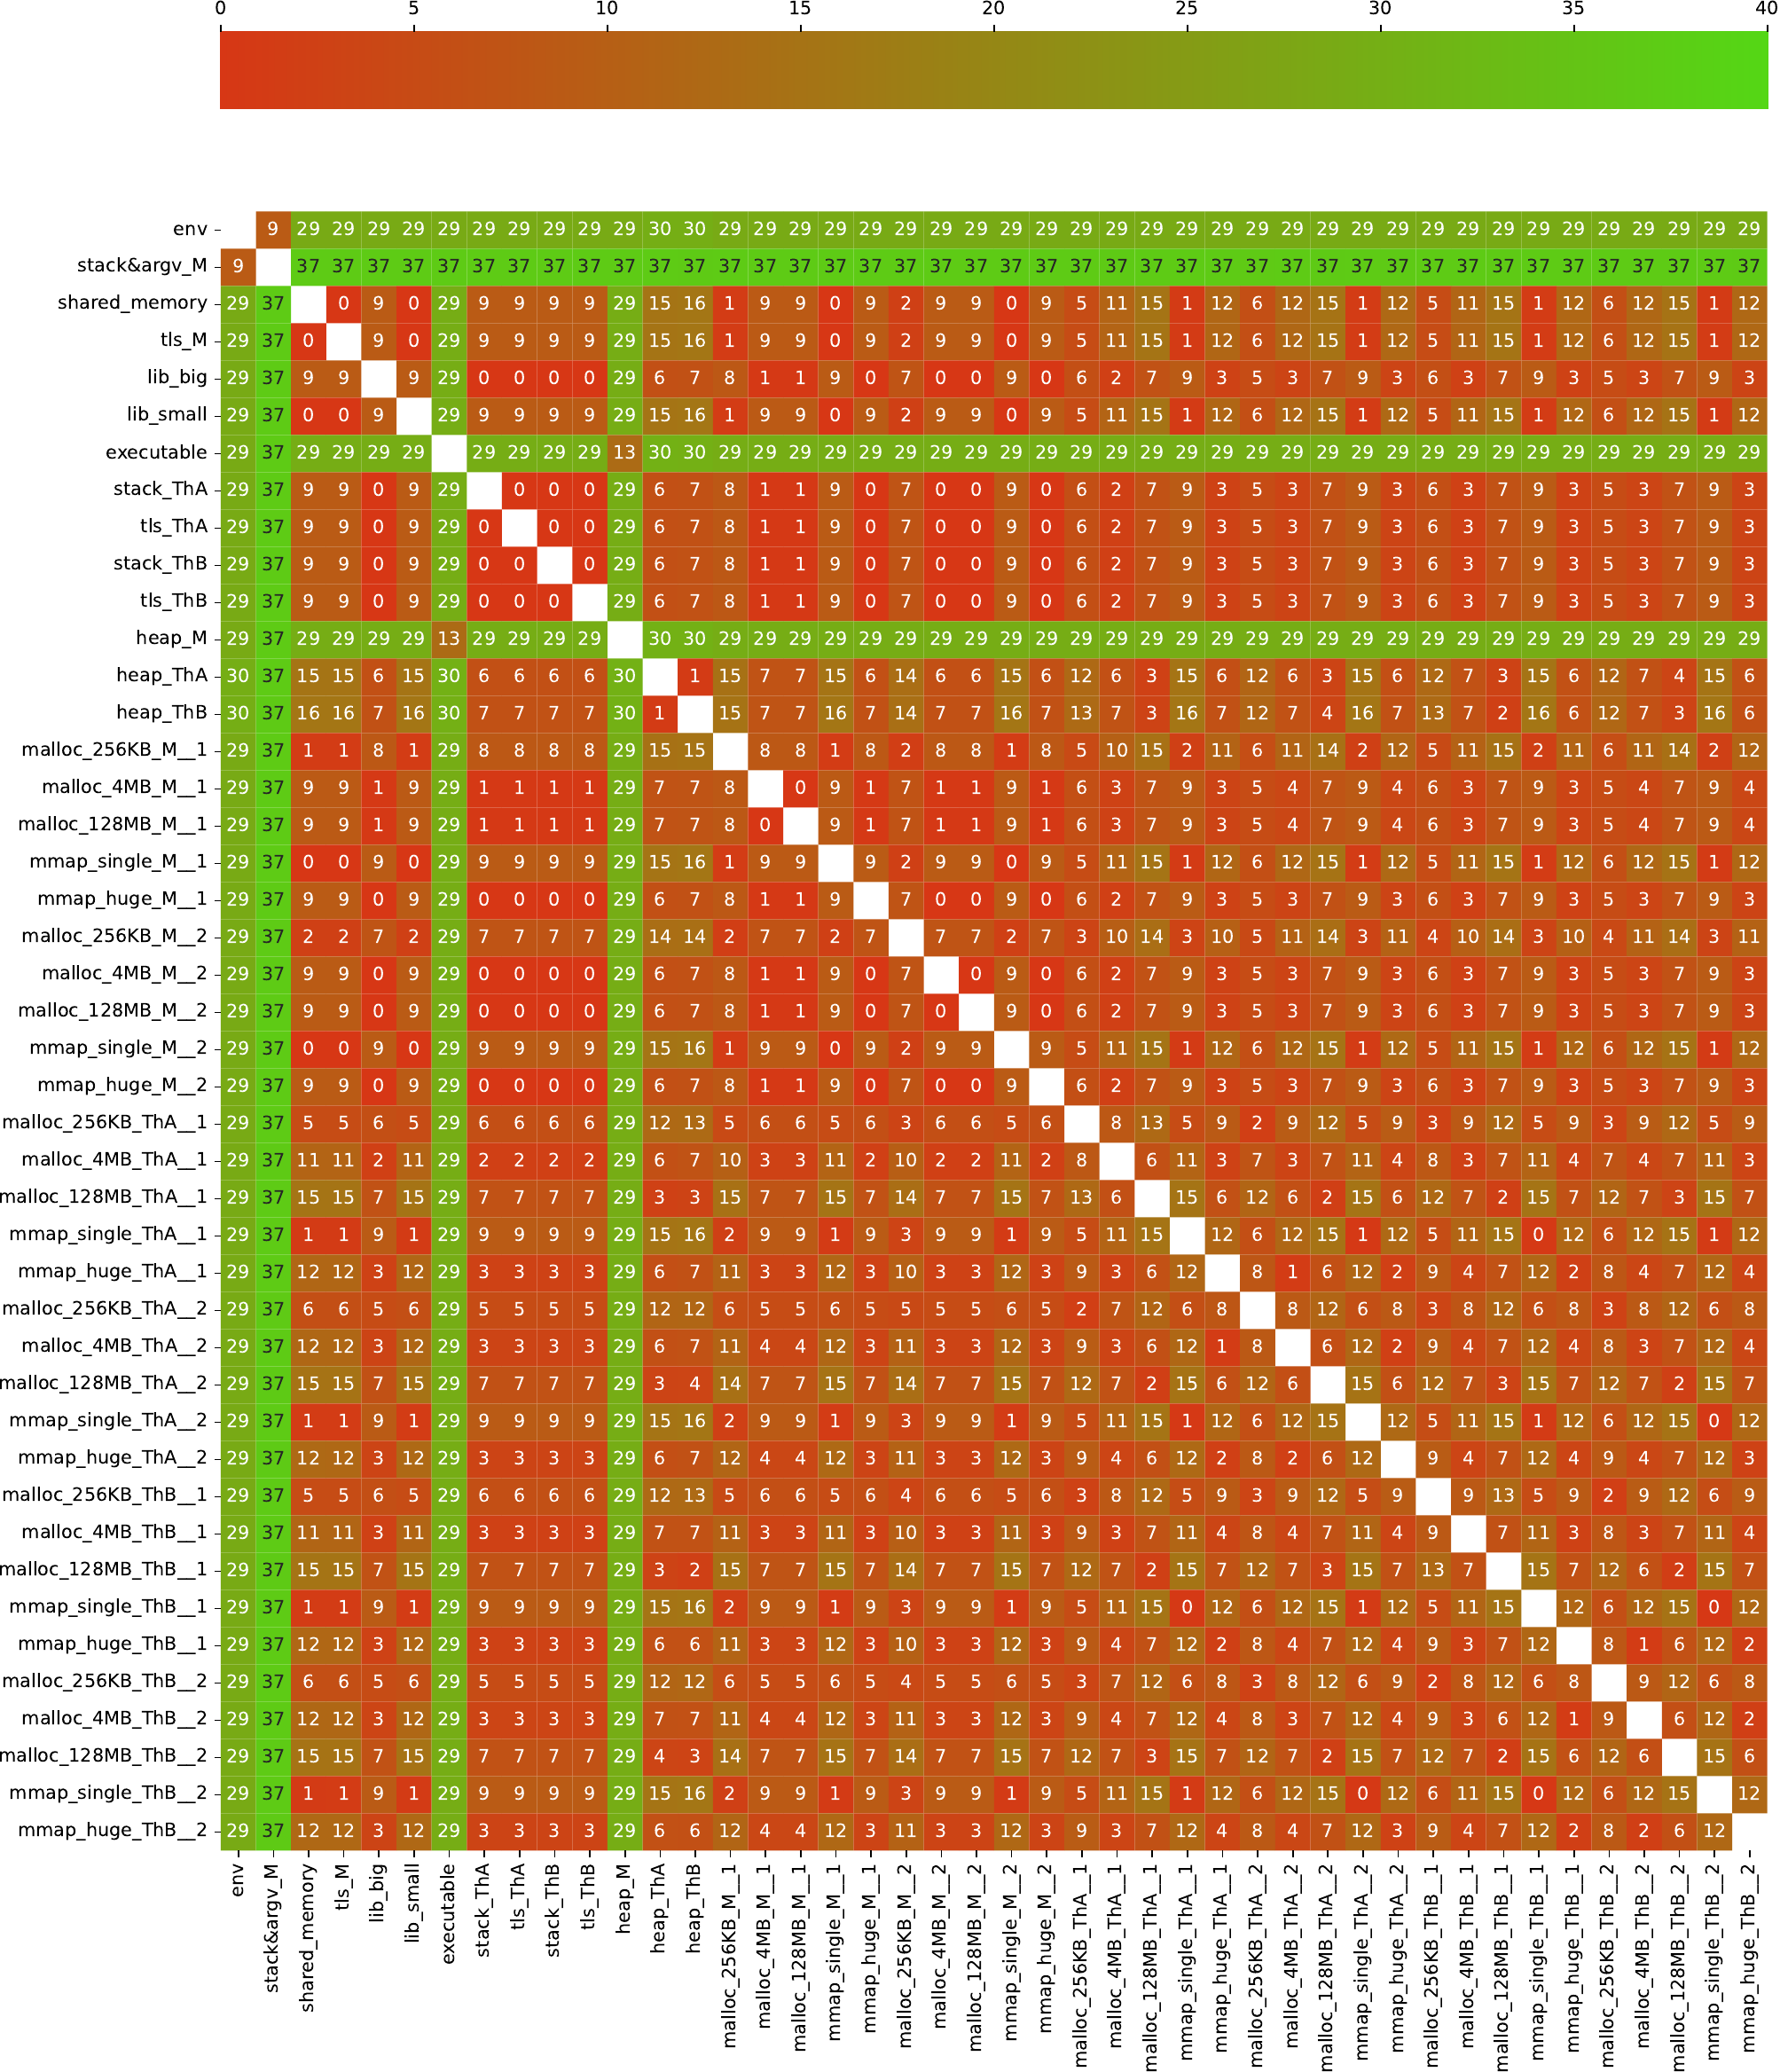}
        \caption{Correlation Entropy Linux 6.4.9}
        \label{fig:corr_lin649}
    \end{subfigure}
    \caption{Correlation Entropy Comparisons Linux}
    \end{adjustwidth}
\end{figure*}
