# Supplementary material for: The Illusion of Randomness: An Empirical Analysis of Address Space Layout Randomization Implementations
Source: arXiv:2408.15107 source file (2024-08-29)
Supplement: Supplementary file 3 [file windows.tex]

\section{Windows Results}

\begin{figure*}[tbh]
    \centering
    \centering
    \includegraphics[width=\textwidth]{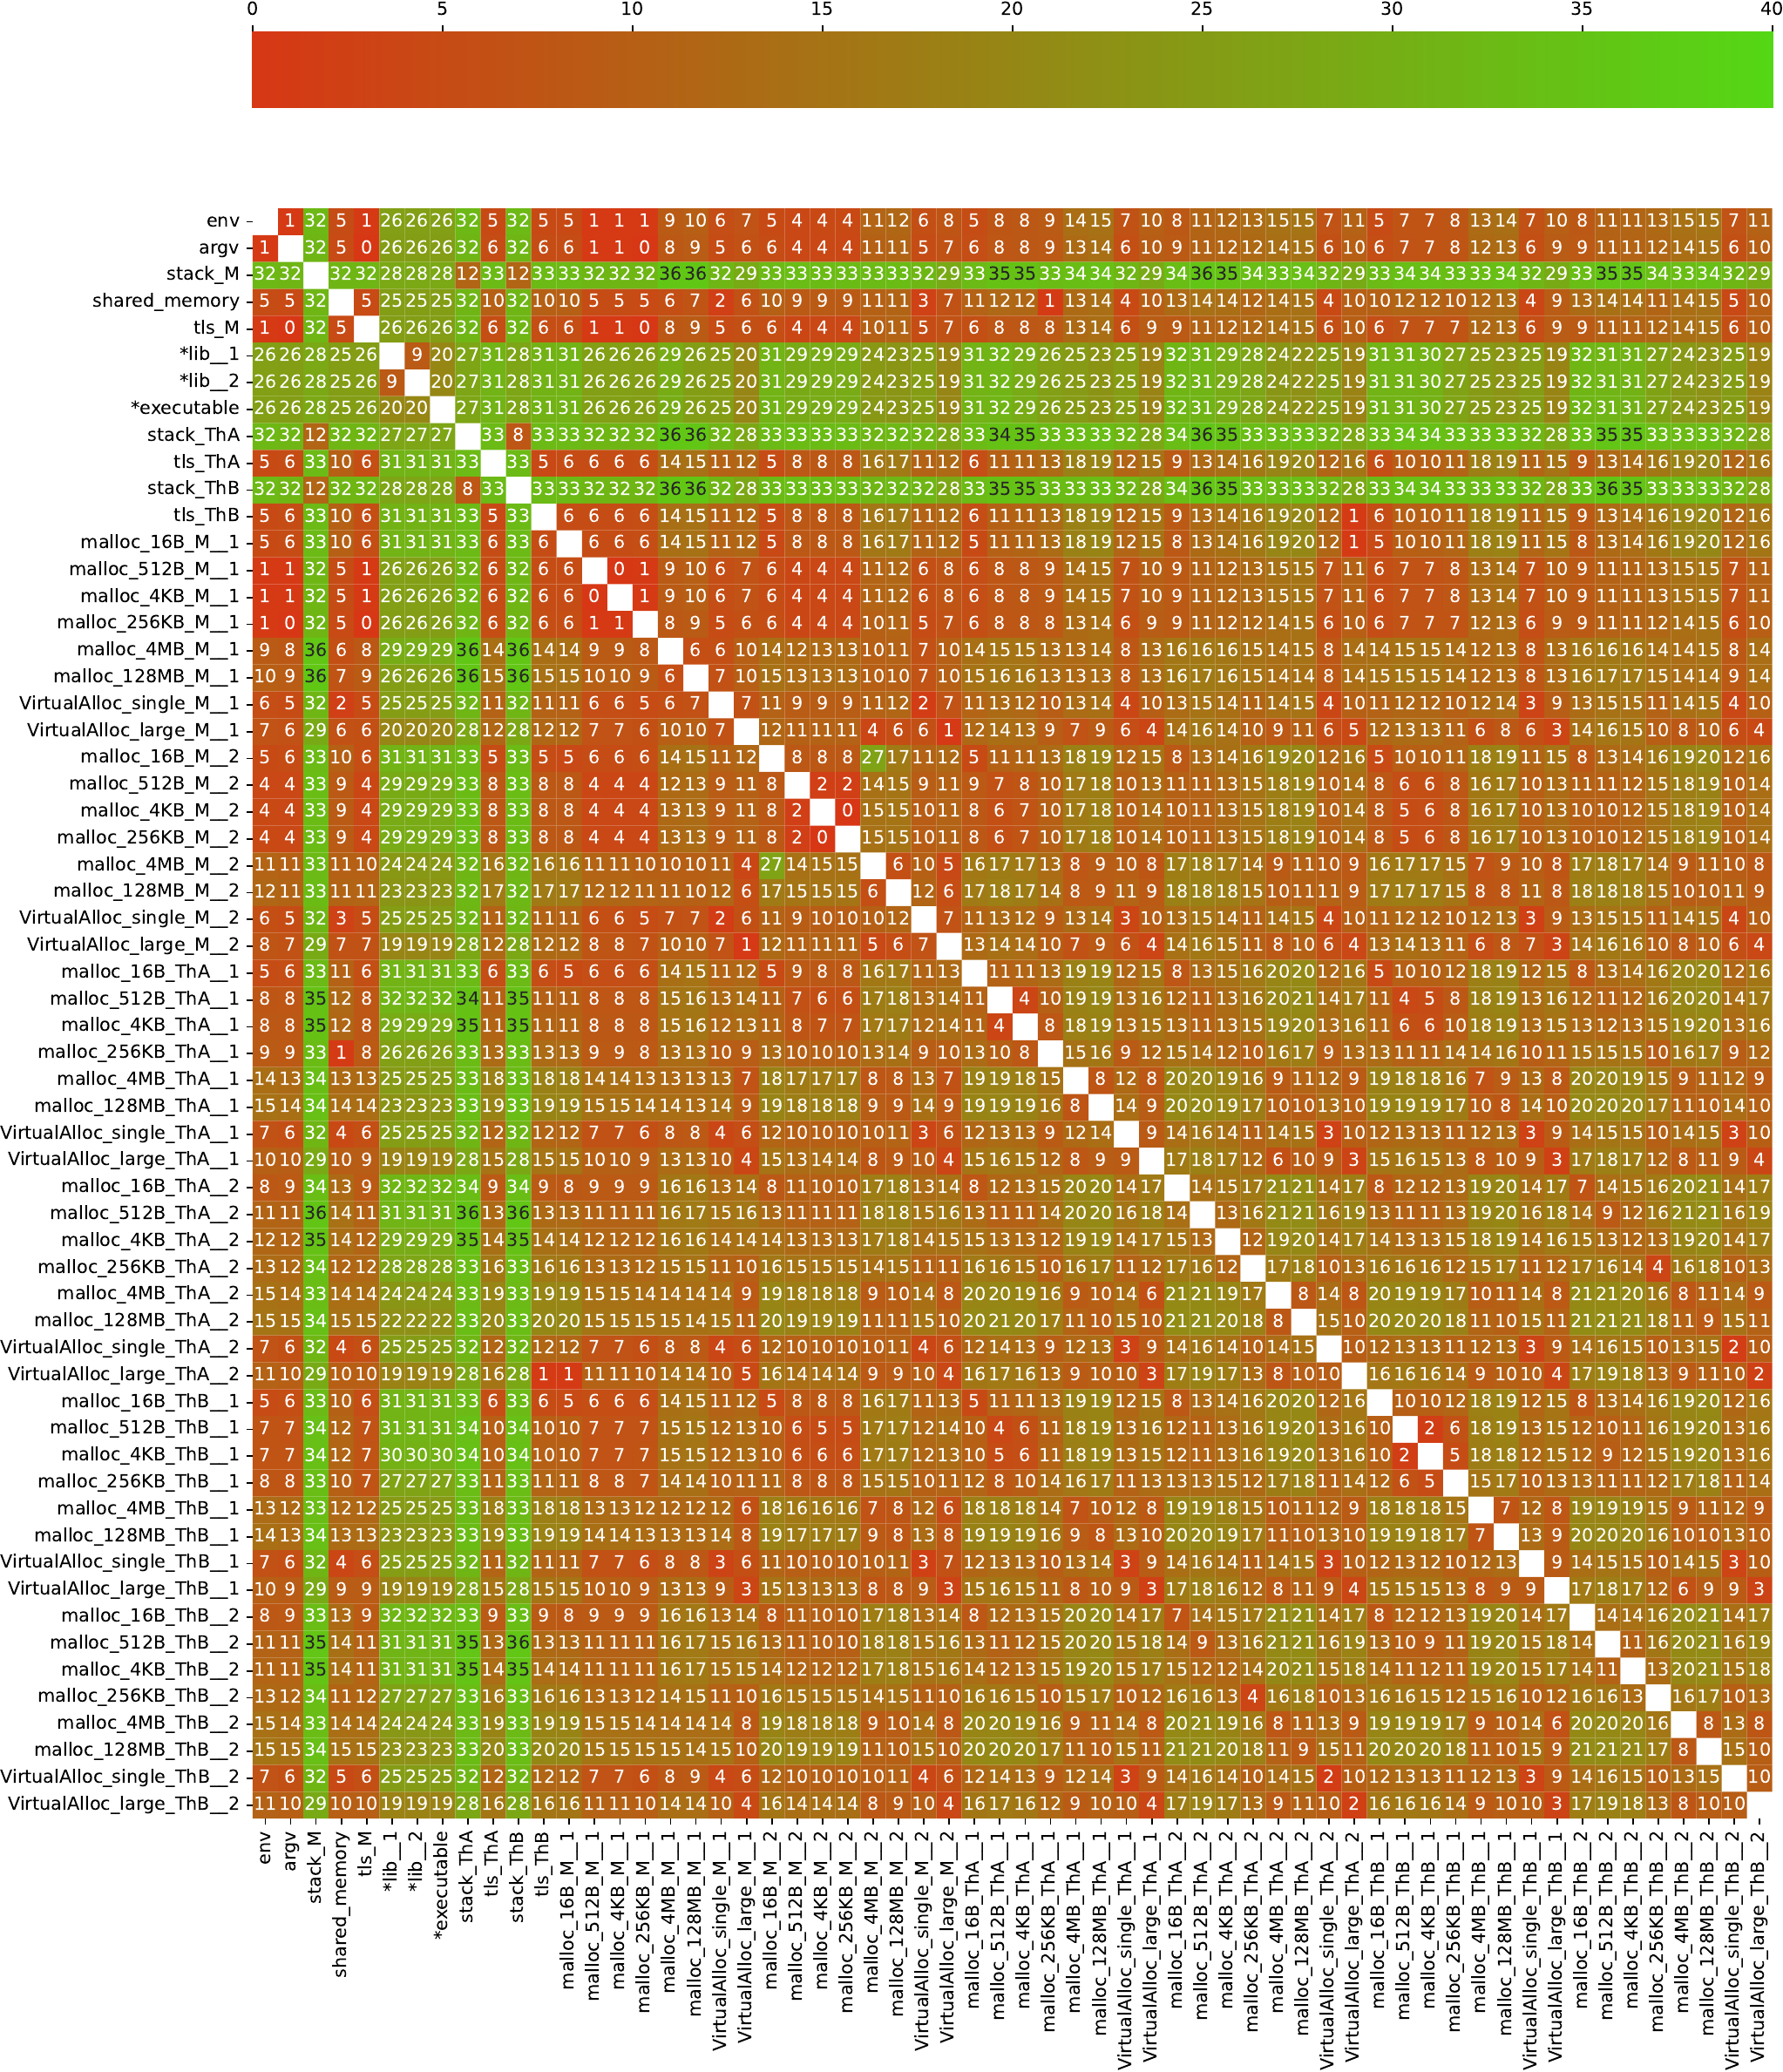}
    \label{fig:corr_lin649}
    \caption{Correlation Entropy Windows 11.}
    \end{adjustwidth}
\end{figure*}
